# Supplementary material for: Persistent Homology with Improved Locality Information for more Effective Delineation
Source: arXiv:2110.06295 source file (2022-12-24)
Supplement: Supplementary file 1 [file supp.tex]

% !TEX root = ../top.tex
% !TEX spellcheck = en-US

\section{Qualitative Results}

The qualitative results for the \MAS{} data set can be found in Fig.~\ref{fig:mass-comp}, the corresponding results for the \RTD{} data set in Fig.~\ref{fig:rtd-comp}, and for the \NEU{} data set in Fig.~\ref{fig:neu-comp}. For each method, we display the thresholded predictions with their skeletons overlaid in red. In the case of the 3D dataset, the images we show are maximum intensity projections.

% !TEX root = ../top.tex
% !TEX spellcheck = en-US

\begin{figure*}[b]
	\centering
	\begin{tabular}{@{} c c c @{}}
		\includegraphics[width=0.3\textwidth]{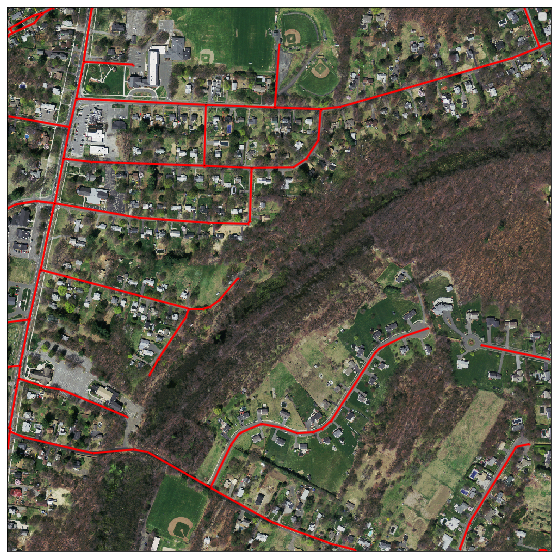} &
		\includegraphics[width=0.3\textwidth]{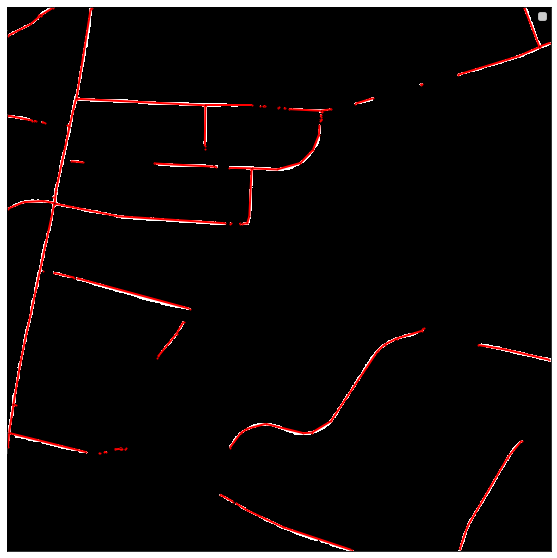} &
		\includegraphics[width=0.3\textwidth]{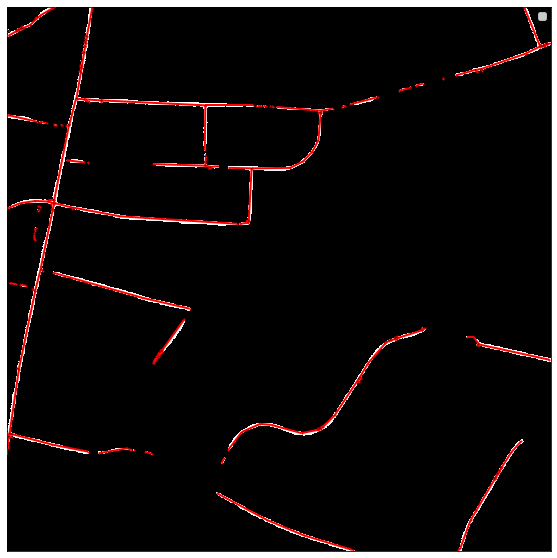} \\
		{\it The input and the ground truth network} &
		\CE{} &
		\MSE{} \\
		
		\includegraphics[width=0.3\textwidth]{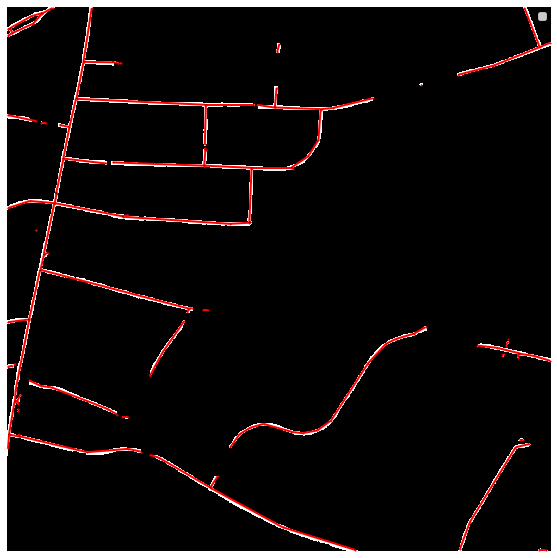} & 
		\includegraphics[width=0.3\textwidth]{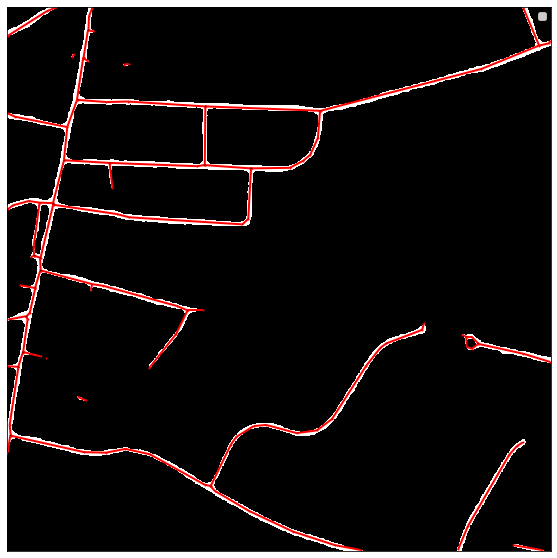} &
		\includegraphics[width=0.3\textwidth]{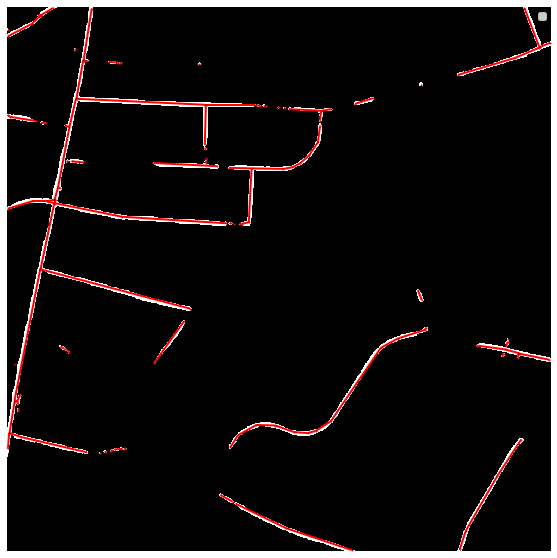}  \\
		\DMT{}& 
		\Malis{} &
		\HomoT{} \\
		
		\includegraphics[width=0.3\textwidth]{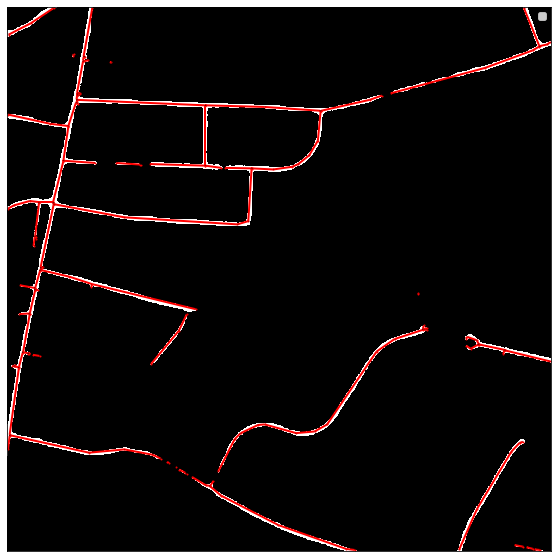} & 
		\includegraphics[width=0.3\textwidth]{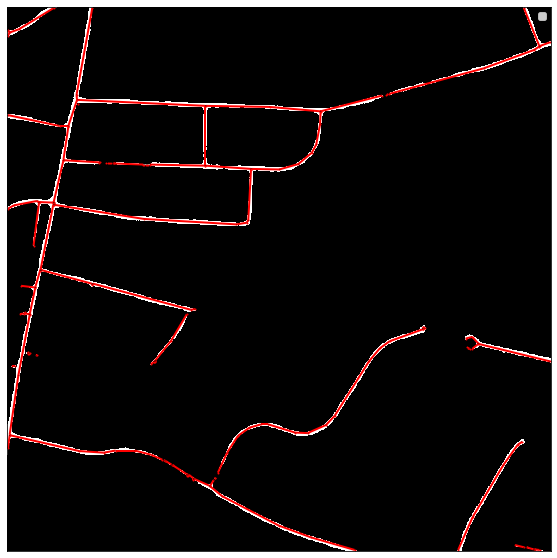} &  \\
		\HomoR{}& 
		\Ours{} & \\
	\end{tabular}
\vspace{-3mm}
\caption{Qualitative results on the \MAS{} dataset.}
\label{fig:mass-comp}
\end{figure*}

% !TEX root = ../top.tex
% !TEX spellcheck = en-US

\begin{figure*}[b]
	\centering
	\begin{tabular}{@{} c c c @{}}
		\includegraphics[width=0.3\textwidth]{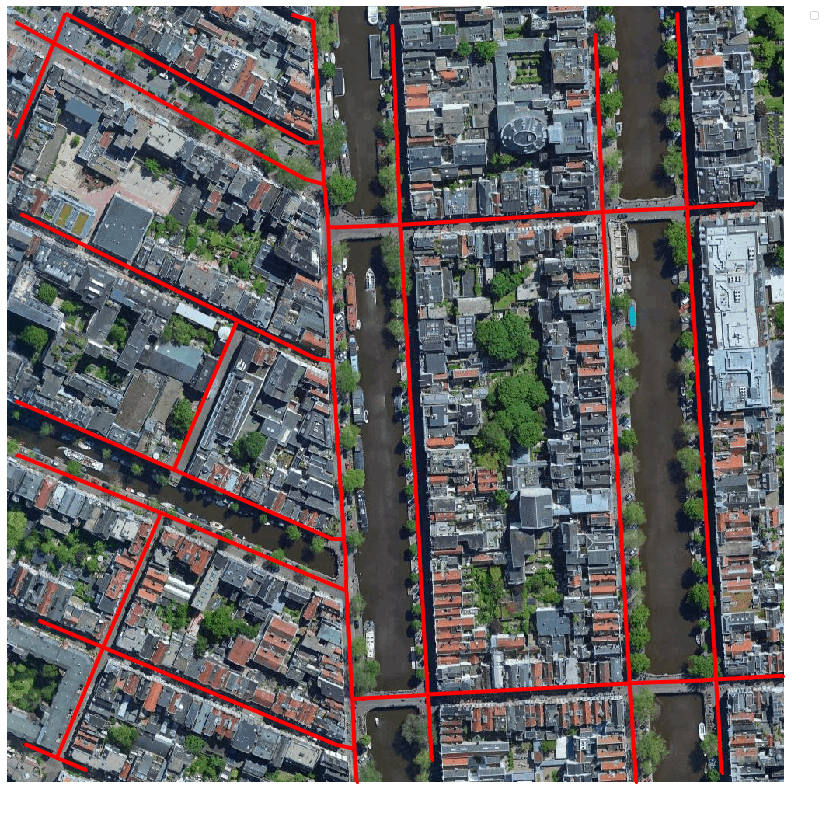} &
		\includegraphics[width=0.3\textwidth]{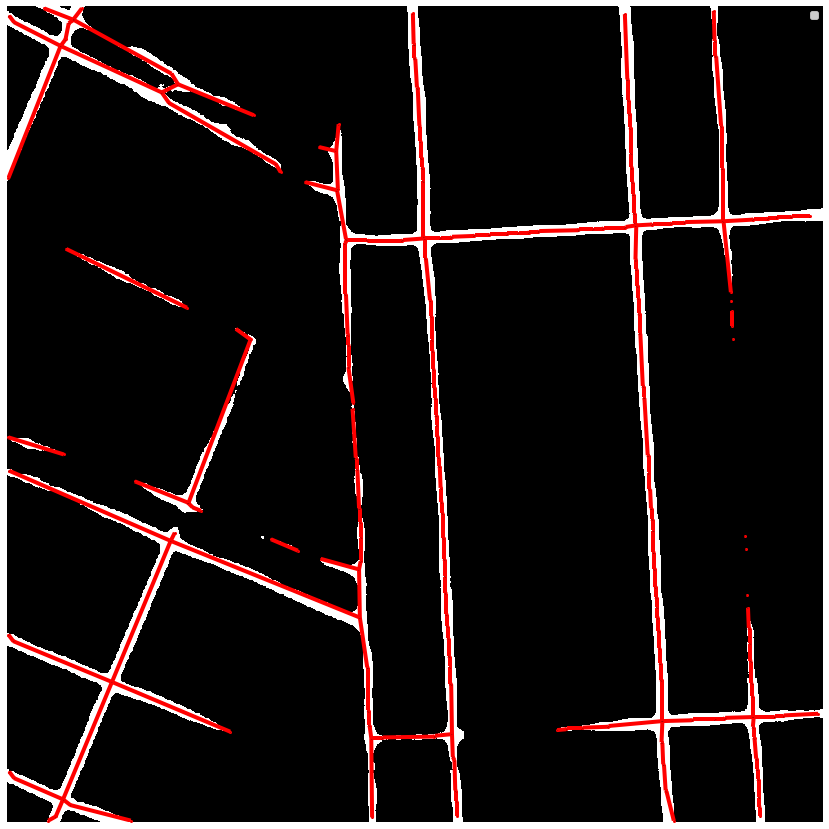} &
		\includegraphics[width=0.3\textwidth]{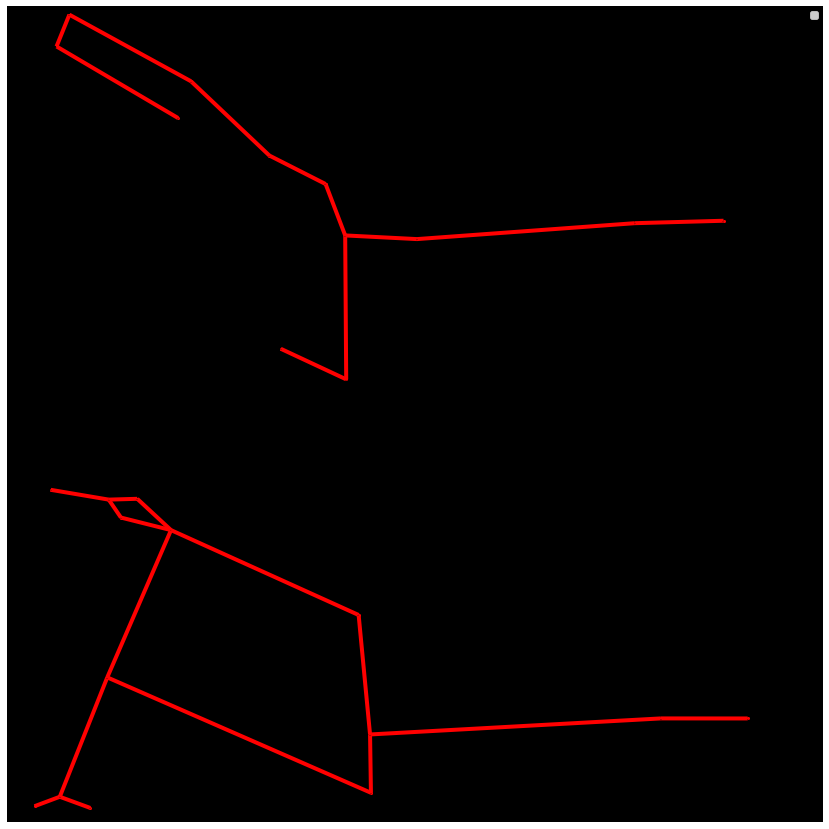} \\
		{\it The input and the ground truth network} &
		\MSE{} &
		\Segm{} \\
		
		\includegraphics[width=0.3\textwidth]{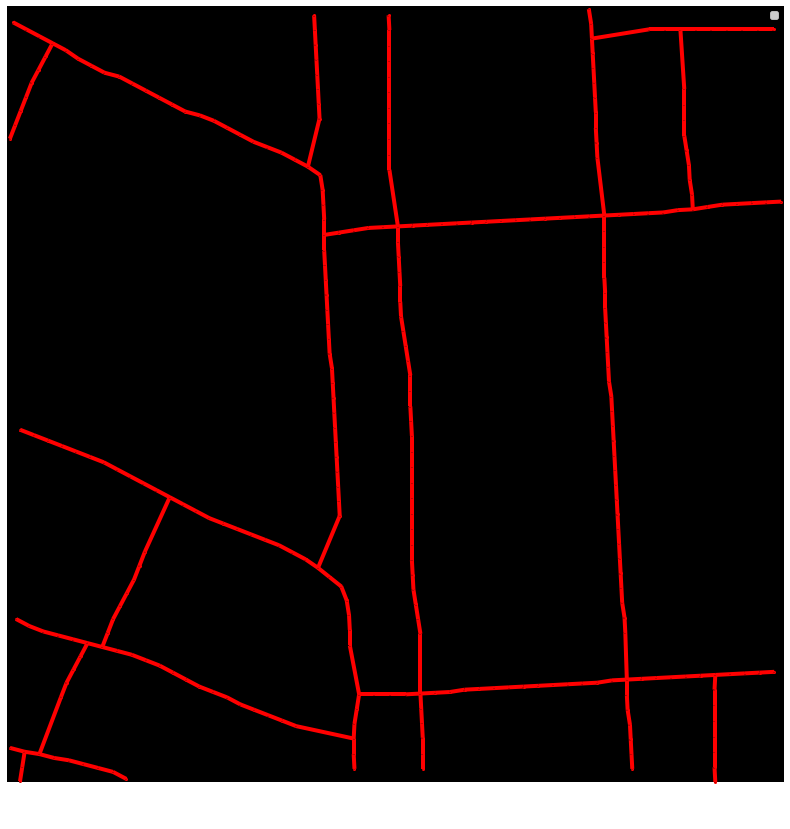} & 
		\includegraphics[width=0.3\textwidth]{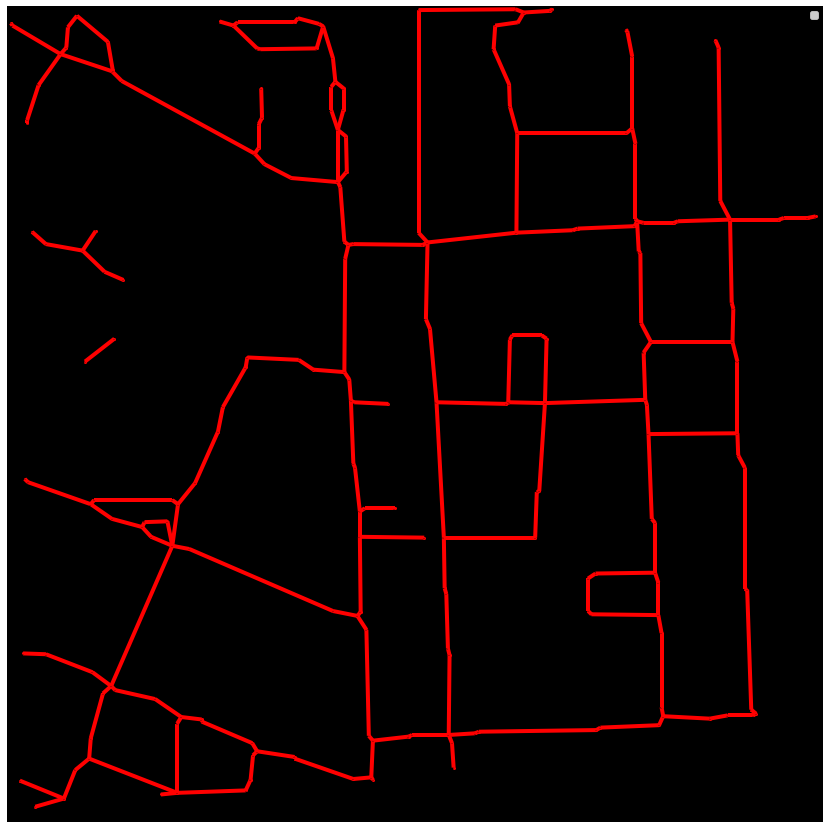} &
		\includegraphics[width=0.3\textwidth]{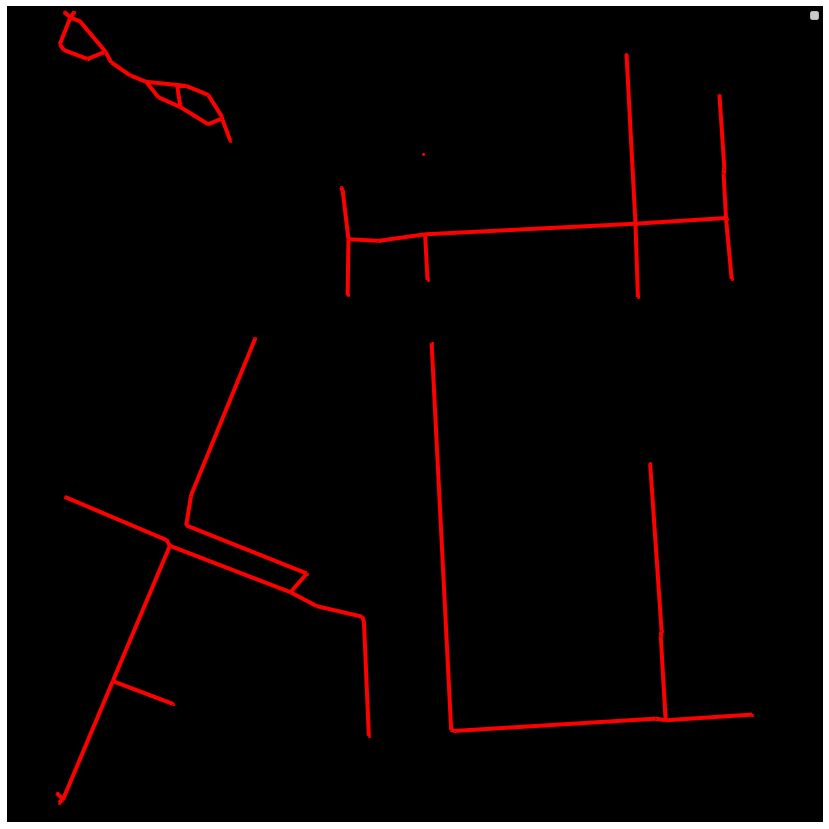}  \\
		\RTracer{}& 
		\SegPath{} &
		\RCNN{} \\
		
		\includegraphics[width=0.3\textwidth]{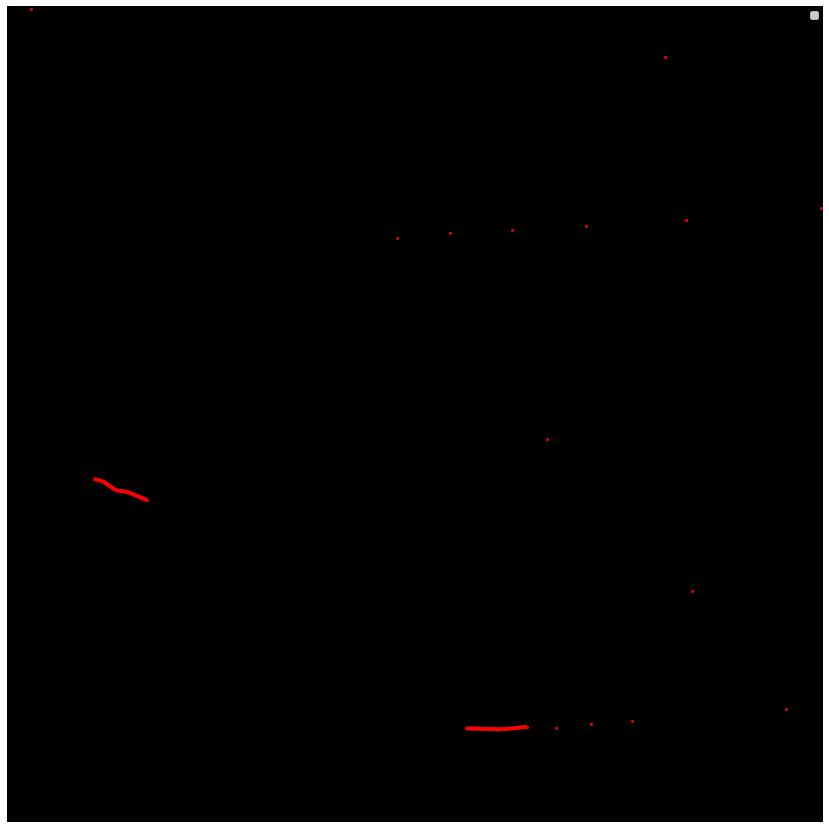} &
		\includegraphics[width=0.3\textwidth]{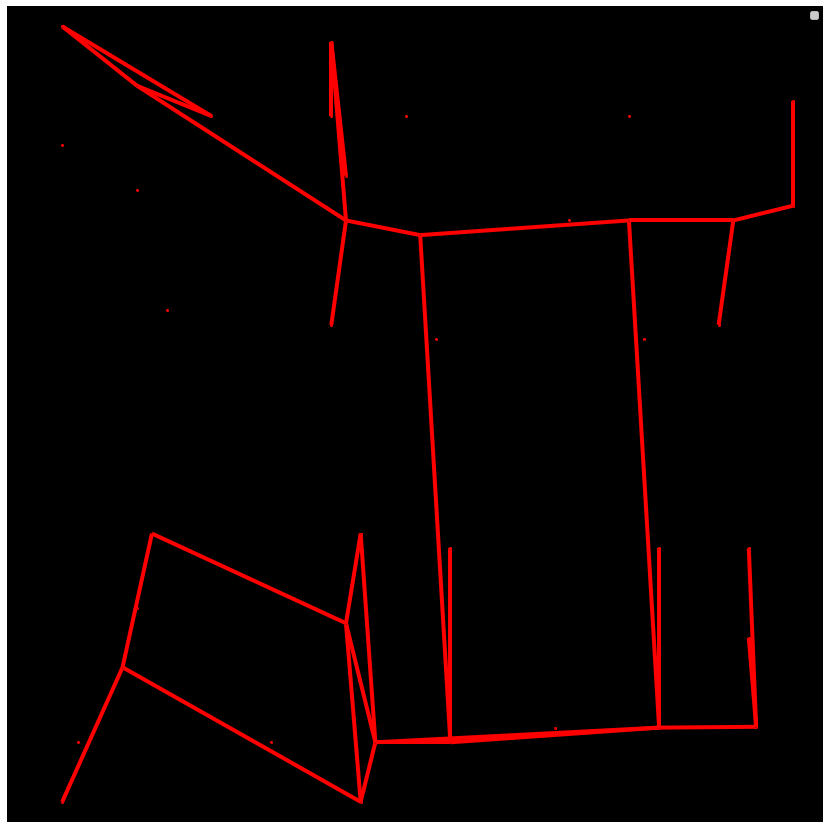} &  
		\includegraphics[width=0.3\textwidth]{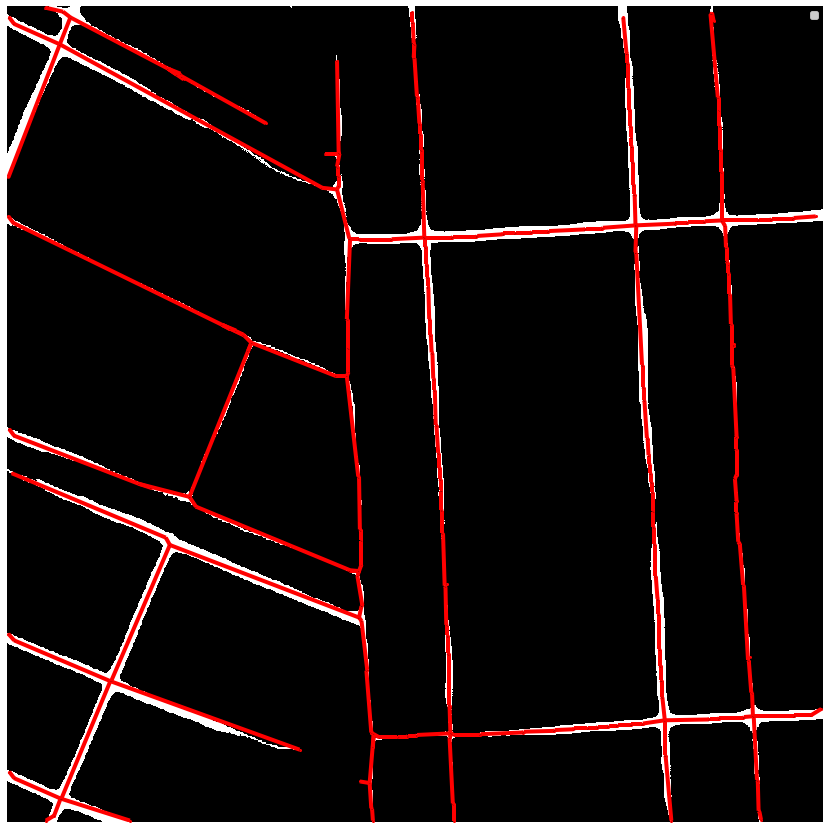}   \\
		\DRoad{}& 
		\PolyM{} &
		\Malis{} \\
	
		\includegraphics[width=0.3\textwidth]{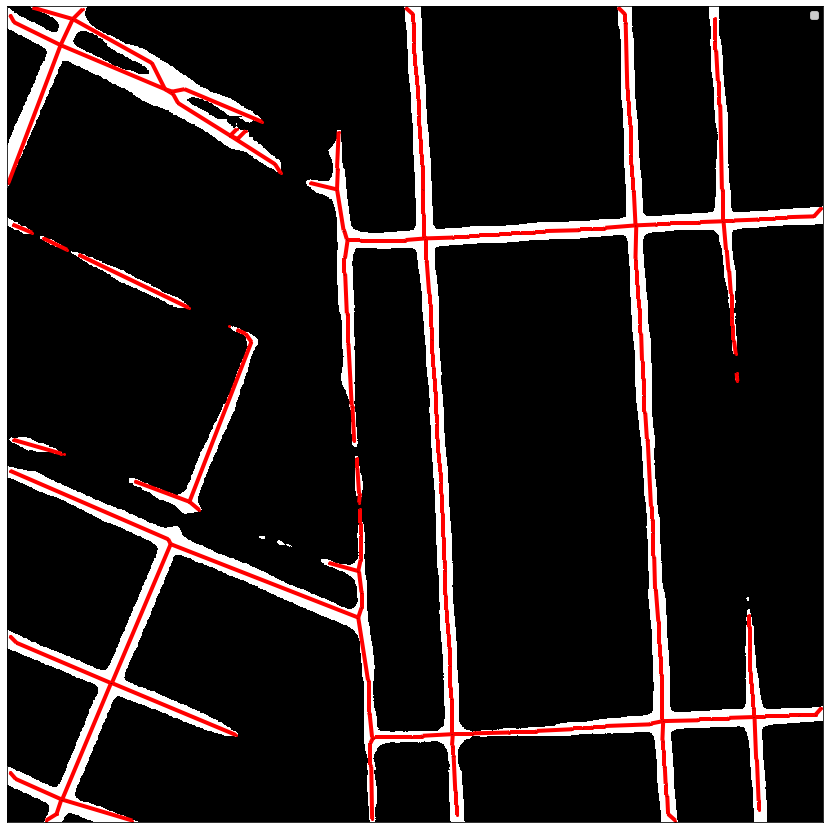} &
		\includegraphics[width=0.3\textwidth]{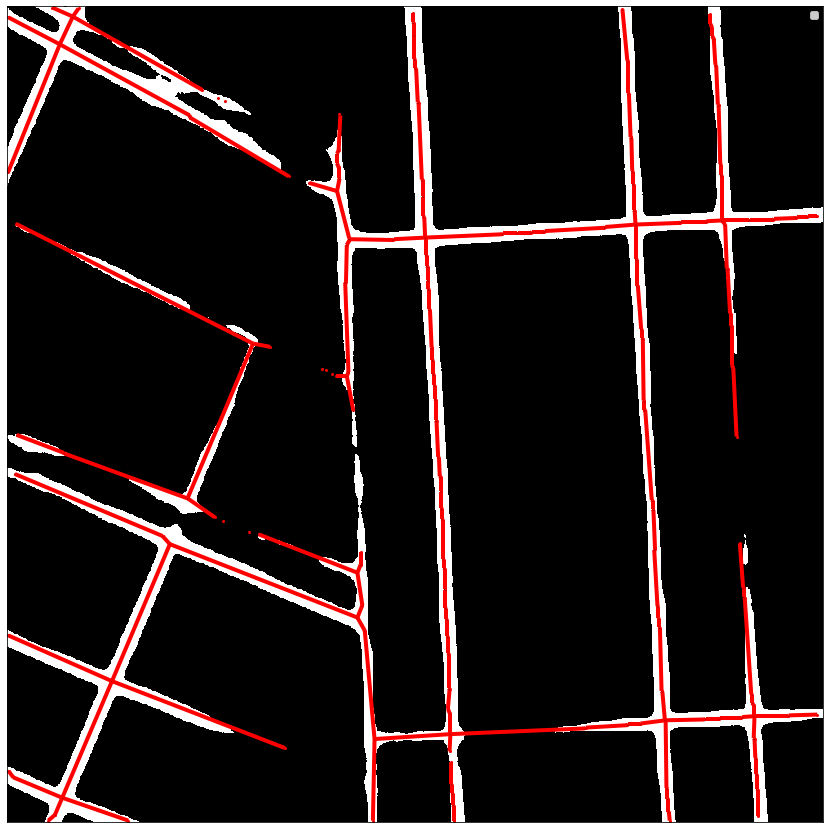} &  
		\includegraphics[width=0.3\textwidth]{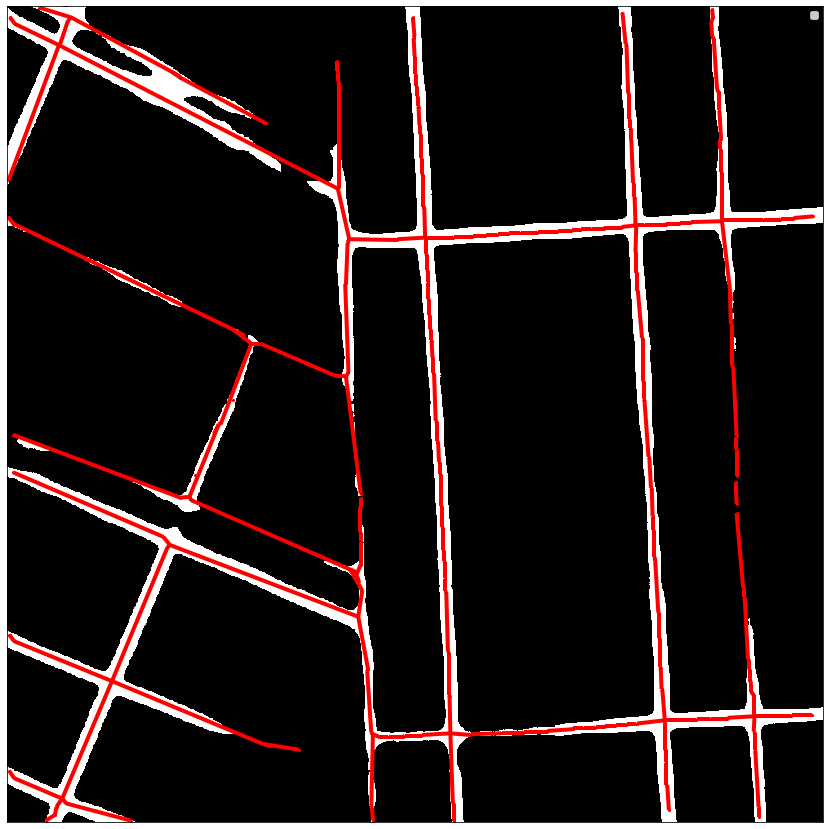}   \\
		\HomoT{}& 
		\HomoR{} &
		\Ours{} \\
	\end{tabular}
\vspace{-3mm}
\caption{Comparative results on the \RTD{} dataset.}
\label{fig:rtd-comp}
\end{figure*}

% !TEX root = ../top.tex
% !TEX spellcheck = en-US

\begin{figure*}
	\centering
	\begin{tabular}{@{} c c c @{}}
		\includegraphics[width=0.3\textwidth]{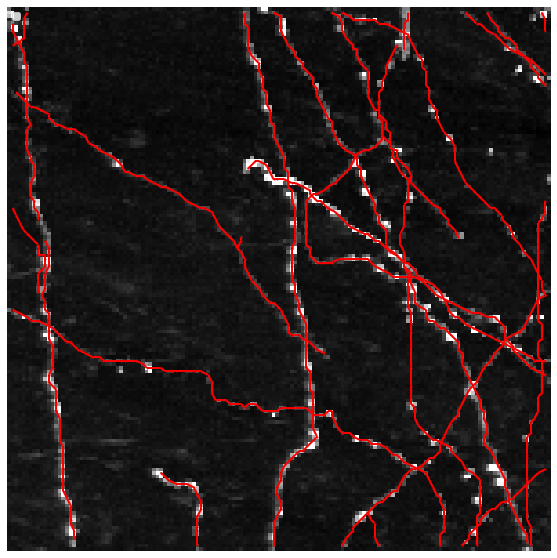} &
		\includegraphics[width=0.3\textwidth]{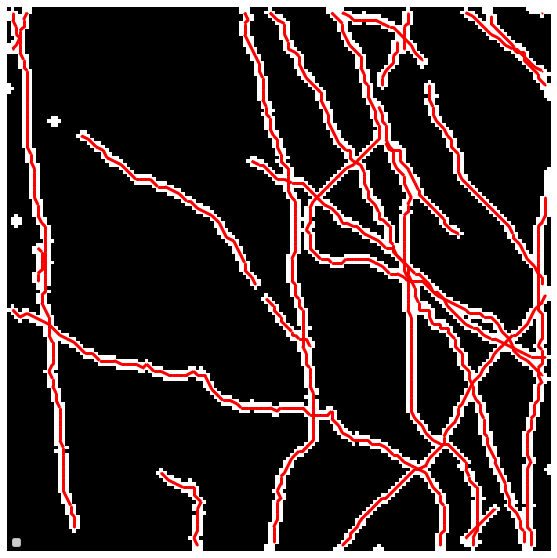} &
		\includegraphics[width=0.3\textwidth]{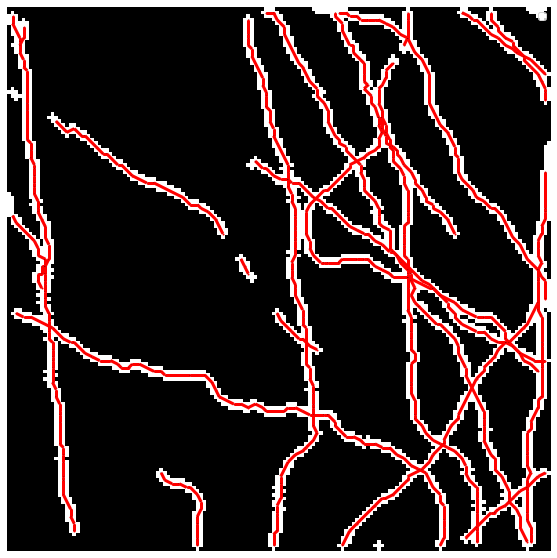} \\
		{\it The input and the ground truth network} &
		\CE{} &
		\MSE{} \\
		
		\includegraphics[width=0.3\textwidth]{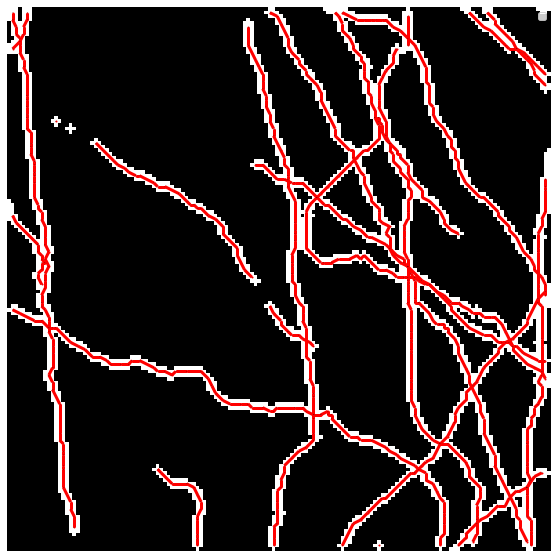} & 
		\includegraphics[width=0.3\textwidth]{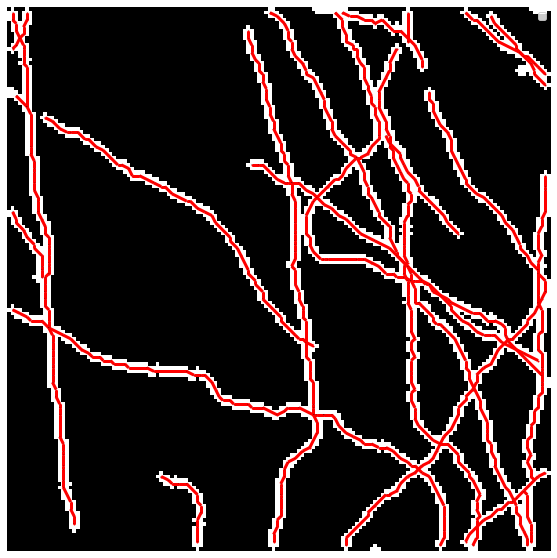} &
		\includegraphics[width=0.3\textwidth]{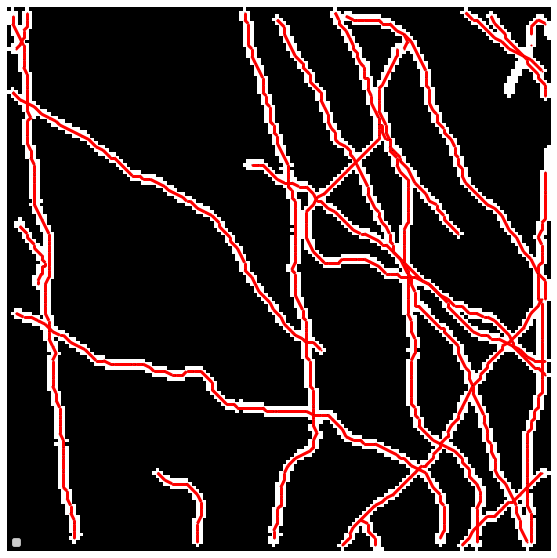}  \\
		\HomoT{}& 
		\HomoR{} &
		\Ours{}
	\end{tabular}
\vspace{-3mm}
\caption{Comparative results on the 3D \NEU{} dataset. }
\label{fig:neu-comp}
\end{figure*}

\section{Ablation Study}

To investigate the impact of hyper-parameter choices on performance, we ran three ablation studies.

% !TEX root = ../top.tex
% !TEX spellcheck = en-US

\begin{table}[!h]
	\centering
	\caption{
		Impact of changing the learning coefficient of localized PH loss on the \MAS{} dataset.
		The window size is fixed to 64x64.
		\label{tab:results-abl-coeff}
	}
	\begin{tabular}{@{} p {0.14\columnwidth} @{}>{\centering\arraybackslash}p{1.0cm}>{\centering\arraybackslash}p{1.0cm}>{\centering\arraybackslash}p{1.0cm} >{\centering\arraybackslash}p{1.0cm}@{}>{\centering\arraybackslash}p{0.2cm}@{}>{\centering\arraybackslash}p{1.4cm} @{} }
		\cmidrule{2-7}
		
		& \multicolumn{4}{c}{Connectivity-oriented} && pixel-based \\
		
		\cmidrule{2-5}
		\cmidrule{7-7}
		
		$\alpha$ &    \APLS{} &       \TLTS &      \Junc &         \Betti &&        \CCQ \\
		\cmidrule{1-7}
		
		1e-3&
		64.9 &    46.0    &    77.1  &  1.21  &&    72.3 \\
		1e-2  & 
		\textbf{68.7} &    \textbf{50.6}    &    \textbf{79.2}  &  \textbf{0.90}  &&    \textbf{74.9} \\
		1e-1&
		67.1 &    48.9     &  77.8   &  0.94  &&    74.6 \\
		1e-0&
		 64.8     &  45.8   &    76.2        &  1.10  &&    72.0 \\
		\cmidrule{1-7}
		
	\end{tabular}
\end{table}

\subsection{Weighting the PH Loss}

We varied the coefficient $\alpha$ in~eq.~(1), while keeping the other parameters fixed.
We report the results in Tab.~\ref{tab:results-abl-coeff}.
The best results are achieved for $\alpha=0.01$, and the performance decreases when $\alpha$ is set ten times higher or lower.
This suggests that the standard Mean Square Loss is still important for overall performance, which is not a surprise, as the gradient of our persistent-homology-based loss is sparse and concentrated at pixels critical for topological correctness.

% !TEX root = ../top.tex
% !TEX spellcheck = en-US

\begin{table}[!h]
	\centering
	\caption{
		Impact of changing the window size when computing our localized loss on the \MAS{} dataset.
		The learning coefficient is fixed to 1e-2.
		\label{tab:results-abl-window}
	}
	\begin{tabular}{@{} p {0.14\columnwidth} @{}>{\centering\arraybackslash}p{1.0cm}>{\centering\arraybackslash}p{1.0cm}>{\centering\arraybackslash}p{1.0cm} >{\centering\arraybackslash}p{1.0cm}@{}>{\centering\arraybackslash}p{0.2cm}@{}>{\centering\arraybackslash}p{1.4cm} @{} }
		\cmidrule{2-7}
		
		& \multicolumn{4}{c}{Connectivity-oriented} && pixel-based \\
		
		\cmidrule{2-5}
		\cmidrule{7-7}
		
		Window Size &    \APLS{} &       \TLTS &      \Junc &         \Betti &&        \CCQ \\
		\cmidrule{1-7}
		
		8x8&
		62.1 &    41.9    &    73.0  &  2.84  &&    67.2 \\
		16x16  & 
		62.7 &    42.4    &    74.5  &  2.09  &&    68.8 \\
		32x32&
		65.4 &    45.7     &  77.1   &  1.17  &&    72.5 \\
		64x64&
		\textbf{68.7} &    \textbf{50.6}    &    \textbf{79.2}  &  \textbf{0.90}  &&    \textbf{74.9} \\
		\cmidrule{1-7}
		
	\end{tabular}
\end{table}

\subsection{Window size}

We changed the size of the window in which the persistent homology is computed. We report the results in Tab.~\ref{tab:results-abl-window}. Our method performs best when using large windows that contain significant portions of the structures of interest. We could not try even larger ones because it would have increased the time needed to detect the homologies and slowed down the training too much. 

% !TEX root = ../top.tex
% !TEX spellcheck = en-US

\begin{table}[!h]
	\centering
	\caption{
		Performances of different height functions used for localized PH loss on the \MAS{} dataset.
		The learning coefficient is fixed to 1e-2 and window size to 64x64
		\label{tab:results-abl-function}
	}
	\begin{tabular}{@{} p {0.22\columnwidth} @{}>{\centering\arraybackslash}p{1.0cm}>{\centering\arraybackslash}p{1.0cm}>{\centering\arraybackslash}p{1.0cm} >{\centering\arraybackslash}p{1.0cm}@{}>{\centering\arraybackslash}p{0.2cm}@{}>{\centering\arraybackslash}p{1.4cm} @{} }
		\cmidrule{2-7}
		
		& \multicolumn{4}{c}{Connectivity-oriented} && pixel-based \\
		
		\cmidrule{2-5}
		\cmidrule{7-7}
		
		Height Function &    \APLS{} &       \TLTS &      \Junc &         \Betti &&        \CCQ \\
		\cmidrule{1-7}
		
		Dist.\ to a point &
		67.8  &    49.4    &   77.9  &  1.01  &&   73.6  \\
		Random Linear &
		\textbf{68.7} &    \textbf{50.6}    &    \textbf{79.2}  &  \textbf{0.90}  &&    \textbf{74.9} \\
		Fixed Linear &
		67.5 &    48.7    &    76.5  &  1.15  &&    73.0 \\
		Square &
		64.2 &    45.1    &    76.3  &  1.32  &&    70.3 \\
		
		\cmidrule{1-7}
		
	\end{tabular}
\end{table}

\subsection{Height Functions}

We also evaluated the effect on performance of using different forms of function $g$ in~eq.~(2), that ties homology birth and death times to image coordinates, distributing the points in the persistence diagram. We present the results in Tab.~\ref{tab:results-abl-function}. The distance to a random image point, or the use of a quadratic instead of linear function of image coordinates do not result in higher performance than the plain linear function.
